# Supplementary material for: Structure Pretraining and Prompt Tuning for Knowledge Graph Transfer
Source: arXiv:2303.03922 source file (2023-03-03)
Supplement: Supplementary file 1 [file experiment-appendix.tex]

\section{Pre-training Details}
We pre-train the {\model} on the latest English version of   ConcepNet\cite{conceptnet}\footnote{https://conceptnet.io/} which includes $1,101,553$ entities, $47$ relations and 2,975,571 triples. We initialize each entity and relation in the embedding table with pre-trained language model BERT\cite{bert}. 
% + 预训练的细节， dimention/layers/每个不同任务的正负样本构造等。。。
\zhu{Our KG pretrain model contains 4 KGTransformer layers with each block having $768$ hidden units and $12$ attention heads. $k$ is set to $126$, that is the length of each sub-graph sequence is shorter than $126$ triples. Due to the disorder of the triples in the sub-graph, we abandoned the position embedding in conventional Transformer.}

\zhu{Given a entity $e$, we generate multiple samples for each task and train them together. For MEM task, we get a sub-graph by random-walk sampling or entity-centered sampling, and 15\% of triples in the sub-graph whose head or tail entities are randomly masked when being serialized into an input sequence. The other entities $e^\prime$ in Equation (5) are randomly sampled from the current training batch and the number of $e^\prime$ for each target entity $e$ is $2$. For MRM task, we get a sub-graph by random-walk sampling or entity-centered sampling, and 15\% of triples in the sub-graph whose relations are randomly masked when being serialized into an input sequence. For EPM task, we first sample a head(tail) entity pair ($e$, $e_j$) with a probability of $50\%$ for entity $e$, where the entity $e_j$ and the entity $e$ used(not used) to be the subject(object) of the same relation. Then the sub-graphs of $e$ and $e_j$ are got by entity-centered sampling, and are serialized and concatenated as an input sequence. The MLPs in Equation (6) and Equation (7) are both 1-layer.}%保证正负样本比例在1：1

\zhu{It is implemented on Pytorch and trained on 1 Tsela-A100 GPU with batch size as $4$ for $9$ epochs. We pretrain the model with Adam whose initial learning rate set at $1e-4$ and use a linear decay learning rate schedule with warm up. Finally the model size is $3.3$G and contains about $875$ million parameters, and the whole training consumed $224$ hours.}

% After pre-train, we apply {\model} to three tasks on benchmark dataset: triple classification on WN18RR, zero-shot image classification on AWA2 and question answering on CommonsenseQA. Statistics of datasets used in experiment are shown in Table \ref{tab:dataset}

% In each task, we compared three settings of {\model} during task tuning:
% % \textit{{\model}} re-uses $\theta_{\mathcal{M}}$ from {\model} and keep them frozen; \textit{{\model}-finetune} tunes $\theta_{\mathcal{M}}$ together with other parameters; \textit{{\model}-scratch} initializes all the parameters and trains the {\model} from scratch. 
% % \begin{itemize}
% %     \item \textit{{\model}} re-uses $\theta_{\mathcal{M}}$ from {\model} and keep them frozen.
% %     \item \textit{{\model}-finetune} tunes $\theta_{\mathcal{M}}$ together with other parameters. 
% %     \item \textit{{\model}-scratch} trains {\model} from scratch, regarding it as a task model.
% % \end{itemize}
% (1) \textit{{\model}} re-uses $\theta_{\mathcal{M}}$ from {\model} and keep them frozen.
% (2) \textit{{\model}-finetune} tunes $\theta_{\mathcal{M}}$ together with other parameters. 
% (3) \textit{{\model}-scratch} trains {\model} from scratch, regarding it as a task model.
% \input{tables/dataset}

\section{Triple Classification Details}
Trained on a knowledge graph $\mathcal{G}$, triple classification model is to predict the correctness given a new triple $\mathcal{D}_{task} = (h,r,t)$.
% \subsubsection{Experiment Details}f
\paragraph{Task Model.}  Applying {\model} to  triple classification, $\mathcal{G}_{task}$ is the concatenation of $h$ and $t$ centered sub-graph, denoted as $\mathcal{G}_h$ and $\mathcal{G}_t$ respectively. The task triple prompt $\mathcal{P}_{task} = [[T]\; [h]\; [r]\; [t] ]$. In the last layer of {\model}, we take out the hidden states correspond to first token $[B]$ and task token $[T]$, denoted as $s_{[B]}^m$ and $s_{[T]}^m$. In the task layer, we concatenate $s_{[B]}^m$ and $s_{[T]}^m$ and input them into a feed forward network and label them $l_{tc}=1$ for positive triple and $l_{tc}=0$ for negative triple. We use a \zhu{Cross-Entropy} loss during training. \zhu{The loss function is
\setcounter{equation}{8}
\begin{equation}
    L_{tc}=\sum_{(h,r,t)\in\mathcal{D}\bigcup\mathcal{D^-}}CE(MLP([s_{[B]}^m||s_{[T]}^m]),l_{tc})
    \label{equ_loss_tc}
\end{equation}
where $\mathcal{D}$ is the positive triple set and $\mathcal{D}^-$ is the negative triple set. }

The detailed overview of triple classification model applying pre-trained KGTransformer is shown in Figure \ref{fig:model-tc}.

\begin{figure}
    \centering
    \includegraphics[width=0.9\textwidth]{figures/model-triple-classification2.pdf}
    \caption{Overview of triple classification model applying pre-trained KGTransformer.}
    \label{fig:model-tc}
\end{figure}

% \paragraph{Dataset}
\paragraph{Training Details.} 
We test and tune {\model} on WN18RR dataset. During tuning, we construct $10$ negative triples by randomly replacing $h$ or $t$ in positive triple $(h,r,t)$. In the test and valid dataset, the number of positive and negative triples are $1:1$. Since entities and relations are different from ConceptNet, %the embedding table are randomly initialized during tuning. 
\zhu{we initialize each entity and relation in the embedding table with pre-trained language model BERT.}
\zhu{We tuning the model with batch size set at 16 and Adam whose initial rate set at $1e-4$, and the MLP in Eqution (\ref{equ_loss_tc}) is 1-layer.}

We compare results of {\model} in different settings to three commonly used knowledge graph embedding methods, TransE\cite{transe}, ComplEx\cite{complex} and RotatE\cite{rotate}, which has proved to be powerful at knowledge graph predictions. 
Following previous works, we train KGEs with link prediction task and after training, we find a proper classification score independently for each relation based on valid dataset. \wen{Specifically, for each relation $r$, we calculate the score of each triple containing relation $r$ in valid dataset, that is $(e, r, e')$. Then we uniformly take $1000$ values between the minimum score and the maximum score as the classification threshold, and take the value achieving the best classification results on valid dataset as the threshold $\gamma_r$ for relation $r$. During test, triples with score larger than $\gamma_r$ are regarded as positive and otherwise as negative ones. }

% \paragraph{Results Analysis.}
% Table \ref{tab:triple-classification} shows the metric of accuracy, precision, recall and F1 score of {\model} in three settings and KGEs. 
% % We analysis table \ref{tab:triple-classification} as follows: 
% Compared to powerful KGEs, {\model} outperforms them and overall achieves the best triple classification results, especially on metrics of Accuracy and F1 score. {\model} is better at recalling positive triples than KGEs and has a reasonable precision on predicted positive triples, thus results the best F1 score. These results prove that {\model} is applicable and effective for triple classification task. 

% Compared to {\model} with frozen tuning setting, overall results of {\model}-finetune is worse, whose averaged accuracy and F1 is $85.5$ while {\model} gives $89.3$, showing the frozen pre-trained {\model} layer introduce a better local minima during tuning which is beyond what could be reached based on task data. This is further supported by comparing {\model} and {\model}-scratch that results of {\model}-scratch are significantly worse than {\model}. 

% % Compared to the results of {\model} with fine-tuning and training from scratch setting, the recommended \wen{frozen {\model} layer tuning} significantly outperforms {\model}-scratch and {\model}-finetune, showing that the pre-trained {\model} helps triples classification.  

\paragraph{Results with Error Bar.} Due to the limitation of space, we only report the main results in the paper. 
Table \ref{tab:tc_eb} show the main results together with error bar of triple classification experiments, which are calculated based on 3 times of experiments.  

% We ran the experiment of each setting 3 times, and the results with error bar are shown in Table \ref{tab:tc_eb}.
\begin{table}[!hbpt]
% \begin{wraptable}{r}{0.6\textwidth}
    \centering
    % \vspace{-6mm}
     \caption{Results with error bar of triple classification on WN18RR\cite{rotate}.}
    \begin{tabular}{l|c c c c}
    \toprule
          & \textbf{Acc.} & \textbf{Precision} & \textbf{Recall} & \textbf{F1}  \\
         \midrule
        TransE \cite{transe} &  88.35 & 93.45 & 82.48 & 87.62  \\ 
        RotatE \cite{rotate} & 88.26 & 93.03 & 82.71 & 87.57 \\
        ComplEx \cite{complex} & 85.07 & 96.73 & 72.59 & 82.94 \\
        \midrule
        \textit{\textbf{\model}}
        % \textbf{KGT}
        & 89.02$\pm$0.08 & 86.66$\pm$0.18 & 92.24$\pm$0.05 & 89.36$\pm$0.05 \\
        \textit{KGT-finetune} &  85.00$\pm$0.20 & 80.85$\pm$0.19 & 91.74$\pm$0.12 & 85.95$\pm$0.14 \\
        \textit{KGT-scratch} & 67.02$\pm$0.16 & 67.91$\pm$0.13 & 64.55$\pm$0.17 & 66.19$\pm$0.15 \\
        \bottomrule
    \end{tabular}
    \label{tab:tc_eb}
% \end{wraptable}
\end{table}

\section{Zero-shot Image Classification Details}
% Zero-shot learning (ZSL) of image classification is a challenging task to train models on samples with \textit{seen classes} while test models on samples with \textit{unseen classes} that have no training samples. 
% Knowledge graph $\mathcal{G}$ usually are used as auxiliary information for augmenting ZSL.  
% \subsubsection{Experiment Details}
\paragraph{Task Model.} 
Applying {\model} to this task, 
we frame the task as outputting the matching score between the input image $I$ and target class $C$. The detailed overview of the zero-shot image classification model applying pre-trained KGTransformer is shown in Figure \ref{fig:model-zsl}.

In this task,  $\mathcal{G}_{task}$ is the class $C$ centered sub-graph $\mathcal{G}_{C}$. The task triple prompt $\mathcal{P}_{task} = [[T]\; [C]\; [M]\; [V]]$ as shown in Figure~\ref{fig:model-zsl}, where $[C]$ is the class token sharing the embedding with entity $C$ in $\mathcal{G}_{task}$; $[M]$ is the mask token indicating relationship between class and image in this task; $[V]$ is the token of current input image whose representation $R_v$ comes from a vision encoder, \zhu{which is transformed through a projection matrix to the same dimension as the input of {\model} as
\begin{equation}
    \mathbf{E}(v)= R_vW_{map}, W_{map}\in\mathbb{R}^{d_{R_v} \times d}
\end{equation}
where $R_v$ is the image representation come from the vision encoder, $\mathbf{E}(v)$ is the representation of current input image before being input to the first {\model} layer.
}

In the last {\model} layer, we take out the hidden state of correspond to the first token $[B]$ and image token $[V]$, denoted as $s_{[B]}^m$ and $s_{[V]}^m$. 
Considering in this task, KG is used to augment unseen classes, we make elements in task triple prompt $P_{task}$ relate with triples in $\mathcal{G}_{task}$ enabling massage aggregating from $\mathcal{G}_{task}$ to $P_{task}$ in {\model} layer while disable the other way by relatedness matrix masking as shown in Figure  \ref{fig:model-zsl}.
In the task layer, 
we project  $s_{[B]}^m$ and $s_{[V]}^m$ through a MLP layer, and then calculate the cosine similarity between them as  
% we calculate the cosine similarity between $MLP(s_{[B]}^m)$ and  $MLP(s_{[V]}^m)$ as 
the matching score of the input image $I$ and class $C$ \zhu{as
\begin{equation}
    score_{(I,C)} = cos\_sim(MLP(s_{[B]}^m),MLP(s_{[V]}^m))
    \label{equ_score_zsl}
\end{equation}
where $cos\_sim(x,y)$ is the cosine similarity of vector $x$ and vector $y$.
}

\zhu{In relatedness matrix, in the line corresponding to the prompt, if the class entity $C$ exists in the triple in the subgraph, the position of the element in the triple is set to 1, and the others are set to 0. In the column corresponding to the prompt, all elements are set to 0. That is, here the visible relationship between the prompt and the subgraph is one-way: the subgraph can directly affect the learning of the prompt representation, but not vice versa.}%在prompt对应的行，如果C实体存在于前面子图中triple中，则该triple对应元素置为1，其他置为0.在prompt对应的列，所有元素置为0.对应实体的的可见性我们定义为：子图中triple包含实体C的才被prompt可见，且prompt不被任何任何三元组可见。即，这里prompt与子图的visible matrix是单向的，即子图可以直接影响prompt的表示，但prompt不直接影响子图表示的学习。

\zhu{We applied BCE loss to encourage the cosine similarity to be large for positive image-class pairs whose label $l_{zsl}=1$ and small for negative image-class pairs whose label $l_{zsl}=0$.}
\zhu{The loss function is
\begin{equation}
L_{zsl}=\sum_{(I,C)\in\mathcal{P}\bigcup\mathcal{P}^-}BCE(\frac{1}{2}(score_{(I,C)}+1),l_{zsl}) 
\label{equ_loss_zsl}
\end{equation}
where $\mathcal{P}$ is the positive image-class pair set and $\mathcal{P}^-$ is the negative image-class pair set; BCE() is the Binary Cross Entropy loss function.}

\begin{figure}
    \centering
    \includegraphics[width=\textwidth]{figures/model-zsl2.pdf}
    \caption{Overview of zero-shot image classification model applying pre-trained KGTransformer.}
    \label{fig:model-zsl}
\end{figure}

% \paragraph{Dataset}
\paragraph{Training Details.}
We tune and test {\model} on AwA-KG benchmark \cite{k-zsl} which includes samples in AwA dataset\cite{awa} and a basic knowledge graph $\mathcal{G}$ containing hierarchy and attributes of 40 seen classes and 10 unseen classes. During tuning, we first train the new embedding table on $G$ with three pre-train tasks and then tune the model with image classification. Following previous works, we use pre-trained  ResNet\cite{resnet} as vision encoder which encode each image into a $2048$ dimensional vector and transform the image vector into $768$ through a trainable transformation matrix and input it to {\model}. During tuning, we froze the parameters in ResNet for simplicity.
% \footnote{Fine-tuning ResNet always present better results according to experience in previous works.}.
\zhu{For each positive pair $(I, C)$, we construct $4$ negative pairs by randomly replacing $C$ with other class $C^\prime$ belongs to 40 seen classes. We tuning the model with batch size set to 12 and Adam whose initial rate set at $1e-4$ and the MLP in Eqution (\ref{equ_score_zsl}) is 1-layer.}

\zhu{When testing, for each test image $I$, we first construct candidate image-class pairs $(I,C_i)$ by pairing the target image $I$ with candidate classes, which is $10$ unseen classes for T1 metric and all $50$ seen and unseen classes for S/U/H metrics,
% all 50 classes $C_i (i = 1,...,50)$, 
and then calculate the scores $score_{(I,C_i)}$ of these candidate pairs by equation (\ref{equ_score_zsl}). Final we sort these scores from high to low, and take $C_i$ in the pair with the highest score as the prediction result. }

\paragraph{Results with Error Bar.} Due to the limitation of space, we only report the main results in the paper. 
Table \ref{tab:zsl_eb} show the main results together with error bar of zero-shot image classification experiments, which are calculated based on 3 times of experiments.
\begin{table}[!hbpt]
% \begin{wraptable}{r}{0.55\textwidth}
    \centering
    \vspace{-3mm}
    \caption{Results with error bar of zero-shot image classification on AwA-KG\cite{k-zsl}}
    \begin{tabular}{l|c| c c c}
    \toprule
        %   \multirow{2}{*}{Method} & ZSL & \multicolumn{3}{c}{GZSL} \\
        % \cline{2-5}
          & \textbf{T1} & \textbf{S} & \textbf{U} & \textbf{H}    \\
         \midrule
        DeViSE\cite{devise} & 43.24 & 86.44 & 6.40 & 11.91  \\ 
        GCNZ\cite{gcnz}  & 62.98 & 75.59 & 20.28 & 31.98 \\
        OntoZSL\cite{ontozsl} & 62.65 & 59.59 & 50.58 & 54.71 \\
        \midrule
        \textit{\textbf{\model}} & 57.38$\pm$0.38 & 63.97$\pm$0.37 & 51.71$\pm$0.32 & 57.19$\pm$0.35 \\
        \textit{KGT-finetune} & 57.65$\pm$0.23 & 62.24$\pm$0.35 & 51.33$\pm$0.34 & 56.26$\pm$0.26 \\
        \textit{KGT-scratch} & 58.96$\pm$0.39 & 56.48$\pm$0.42 & 47.93$\pm$0.27 & 51.85$\pm$0.34 \\
        \bottomrule
    \end{tabular}
    \label{tab:zsl_eb}
    \vspace{-3mm}
% \end{wraptable}
\end{table}

\section{Question Answering Details}
\begin{figure}
    \centering
    \includegraphics[width=\textwidth]{figures/model-QA2.pdf}
    \caption{Overview of question answering model applying pre-trained KGTransformer.}
    \label{fig:model-qa}
\end{figure}

% Question answering is a task to select the correct answer given a natural language question. It is a challenging task requiring complex reasoning over constraints stated in the question in consistent to the  relevant knowledge in the world. Thus knowledge graph $\mathcal{G}$ are used to provide  commonsense background knowledge  for question answering. 

% \subsubsection{Experiment Details}
\paragraph{Task Model.}
Applying {\model} to question answering, we frame the task as output the likelihood of the input question-answer pair to be correct. 
In this task, given a question-choice pair $qc$, we extract  $\mathcal{G}_{task}$ from ConceptNet according to the set of key words $\mathcal{W}$ in $qc$ following \cite{qagnn}. 
The task prompt $\mathcal{P}_{task} = [[T]\; [M] \; [M]\; [Q]]$ as shown in Figure~\ref{fig:model-qa} where $[M]$ is mask token for head entity and relation, and $[Q]$ is the token for current task pair $qc$ whose representation $R_{qc}$ come from a language encoder, \zhu{which is transformed through a projection matrix to the same dimension as the input of {\model} as
\begin{equation}
    \mathbf{E}(qa)= R_{qa}W_{map}, W_{map}\in\mathbb{R}^{d_{R_{qa}} \times d}
\end{equation}
where $R_{qc}$ is the question-choice pair representation come from the language encoder, $\mathbf{E}(qa)$ is the representation of current task pair $qc$ before being input to the first {\model} layer.
}

In the last {\model} layer, we take out the hidden state corresponding to the first token and question-answer pair token, denoted as $s_{[B]}^m$ and $s_{[Q]}^m$. Following \cite{qagnn}, in the task layer, we concatenate $R_{qa}, s_{[B]^m}$ and $s_{[Q]}^m$ and input them into a $MLP$ layer to output the score of $qc$ pair \zhu{as
\begin{equation}
score_{qa} = MLP([s_{[B]}^m||s_{[Q]^m}||R_{qc}])
    \label{equ_score_qa}
\end{equation}
} \zhu{We label the positive pair $l_{qc}=1$ and the  negative pair $l_{qc}=0$. We use a Cross-Entropy loss during training. The loss function is
\begin{equation}
    L_{qc}=\sum_{qa\in\mathcal{P}_{qc}\bigcup\mathcal{P}_{qc}^-}CE(score_{qc},l_{qc})
    \label{equ_loss_qa}
\end{equation}
where $\mathcal{P}_{qc}$ is the positive $qc$ pair set and $\mathcal{P}_{qc}^-$ is the negative pair set.}

The detailed overview of question answering model applying pre-trained KGTransformer is shown in Figure \ref{fig:model-qa}.

% \paragraph{Dataset}
\paragraph{Training Details.}
We tune and test {\model} on CommonsenQA benchmark\cite{commonsenseqa} which is a 5-way multiple choice QA task containing 12,102 questions. We report the main results on the in-house (IH) data splits and official test set as did in \cite{qagnn}. We apply  RoBERTa-large\cite{roberta} as language encoder. 
For each $qc$, RoBERTa output a $1024$ dimensional vector corresponding to $[B]$ token as the representation of $qc$. We transform the representation into $d$ dimensional through a transformation matrix. 
In this task, we regard task triple prompt and a triple in $\mathcal{G}_{task}$ containing key words in $\mathcal{W}$ used to extract knowledge graph as sharing elements during relatedness matrix construction. 
% + 实验细节
\zhu{We tuning the model with batch size set to $128$ and mini batch size set to $4$ and Adam whose initial rate set at $1e-5$ and the MLP in Eqution (\ref{equ_score_qa}) is 1-layer. In the first $4$ training epochs, the RoBERTa-large is fixed.}

\zhu{When testing, for each question $q$ and its $5$ choices $c_i (i=1,...,5)$, we calculate the scores $score_{qc_i}$ of the $5$ $qc$ pairs by equation (\ref{equ_score_qa}). Final we sort these scores from high to low, and take $c_i$ in the pair with the highest score as the prediction result.}

% \paragraph{Results Analysis}
% We ran the experiment of each setting 3 times, and the results are shown in Table
% \ref{tab:qa_eb}.

% Due to the limitation of space, we only report the main results in the paper. 
\paragraph{Results with Error Bar.}  Table \ref{tab:qa_eb} show the main results together with error bar of question answering experiments, which are calculated based on 3 times of experiments.

\begin{table}[!hbpt]
% \begin{wraptable}{r}{0.5\textwidth}
% \renewcommand\arraystretch{1.1}
\centering
% \vspace{-5mm}
\caption{Accuracy with error bar of QA on CommonsenseQA. 
% Results of baselines are taken from \cite{qagnn}
}
% \resizebox{\columnwidth}{!}{
\begin{tabular}{lcc}
\toprule
& \textbf{IHdev} & \textbf{IHtest} \\
\midrule
% RoBERTa-large\cite{roberta} & 73.07 ($\pm$.45) & 68.69 ($\pm$.56) \\ 
% \midrule
% + RGCN\cite{rgcn}   & 72.69 ($\pm$.19) & 68.41 ($\pm$.66) \\
% + GconAttn\cite{DBLP:conf/aaai/WangKMYTACFMMW19} & 72.61 ($\pm$.39) & 68.59 ($\pm$.96) \\
% + KagNet\cite{DBLP:conf/emnlp/LinCCR19}   & 73.47 ($\pm$.22) & 69.01 ($\pm$.76) \\
% + RN\cite{DBLP:conf/nips/SantoroRBMPBL17}       & 74.57 ($\pm$.91) & 69.08 ($\pm$.21) \\
% + MHGRN\cite{DBLP:conf/emnlp/FengCLWYR20}    & 74.45 ($\pm$.10) & 71.11 ($\pm$.81) \\
% + QA-GNN\cite{qagnn}   & 76.54 ($\pm$.21) & 73.41 ($\pm$.92) \\
% + GREASELM\cite{greaselm} & 78.50 ($\pm$.50) & 74.20 ($\pm$.40) \\
% + MorsE\cite{morse} & 77.67 ($\pm$.34) & 75.56 ($\pm$.21) \\
RoBERTa-L \cite{roberta} & 73.07 ($\pm$.45) & 68.69 ($\pm$.56) \\ 
RoBERTa-L \cite{roberta}(ours) &  72.17 ($\pm$.06) & 68.49 ($\pm$.07) \\
\midrule
% + RGCN\cite{rgcn}   & 72.69 & 68.41 \\
+ GconAttn \cite{DBLP:conf/aaai/WangKMYTACFMMW19} & 72.61 ($\pm$.39) & 68.59 ($\pm$.96) \\
+ KagNet \cite{DBLP:conf/emnlp/LinCCR19}   & 73.47 ($\pm$.22) & 69.01 ($\pm$.76) \\
% + RN\cite{DBLP:conf/nips/SantoroRBMPBL17}       & 74.57 & 69.08 \\
+ MHGRN \cite{DBLP:conf/emnlp/FengCLWYR20}   & 74.45 ($\pm$.10) & 71.11 ($\pm$.81)  \\
+ QA-GNN \cite{qagnn}   & 76.54 ($\pm$.21) & 73.41 ($\pm$.92) \\
\midrule
+ \textit{\textbf{\model}} & 73.76 ($\pm$.05) & 70.62 ($\pm$.07)\\ 
+ \textit{KGT-finetune} & 73.46 ($\pm$.07) & 70.04 ($\pm$.05)\\ 
+ \textit{KGT-scratch}  & 72.32 ($\pm$.05) & 69.18 ($\pm$.08)\\ 
\bottomrule
\end{tabular}
\label{tab:qa_eb}
% \vspace{-4mm}
% \end{wraptable}
\end{table}

\section{Source Code}
Experiment code are included in the supplementary material.
